# Supplementary material for: Probing Ultrafast Magnetic-Field Generation by Current Filamentation Instability in Femtosecond Relativistic Laser-Matter Interactions
Source: arXiv:1907.12052 source file (2019-07-28)
Supplement: Supplementary file 1 [file Supplemental.pdf]

In Fig. 1, we show the effect of changing the preplasma length on the generation of Weibel-like magnetic field structures. For the Al foil with a flat surface (Fig. 1(a)) the magnetic field strength is found to be higher compared to the case where a preplasma of length $\lambda_0$ (Fig. 1(b)) or $2\lambda_0$ (Fig. 1(c)) is considered. However, for the flat surface case, the length of magnetic field filaments is much shorter than the case with preplasma. The integrated $B_y$ field values in Fig. 1, as calculated for the three cases, are 0.61 kT $\mu$m (flat surface), 0.70 kT $\mu$m (preplasma of $\lambda_0$) and 0.67 kT $\mu$m (preplasma of $2\lambda_0$). This shows that the integrated $B_y$ field experienced by the relativistic electrons does not vary significantly with the increase in preplasma length. This is explained by the compensation between the decreased magnetic field and increased filament length when comparing the case with preplasma to the flat surface case. Because of this weak dependence of the integrated $B$-field with the preplasma length, the knowledge of the exact nature of the preplasma in experiments is not necessary to reasonably predict the observed effect on the electron beam probe.

There are several mechanisms that can generate strong electromagnetic fields in the vicinity of the front surface of the foil, e.g. electron surface wave (ESW), TNSA induction, or Weibel-like current filamentation instability. Figure 2 shows that in the case of a high intensity laser pulse impinging on the solid target ($a_0 = 10$), strong transverse surface ripples or modulations are observed, with a wavelength of $\approx 110$ nm, in both the electron (Fig. 2(e)) and ion (Fig. 2(f)) densities. Such surface modulations (which can seed Rayleigh Taylor instabilities) have been used to explain the transverse mesh like structures in the proton beam profiles obtained during the target normal sheath acceleration (TNSA) experiments [1-2]. The TNSA regime is characterized by significantly higher energy lasers (*i.e.* longer duration or higher intensity or both) and typically thin ($2-3$ $\mu$m) solid targets. However, in our regime of investigation, with femtosecond and moderately relativistic laser pulses (estimated $a_0$ ranging from 2.3 to 0.7), we do not observe any surface modulations in the electron or ion density profiles (see Figs. 2(b) and (c)). The observed spatial modulation of the current is source for the magnetic-field fluctuations, and originates from the unstable anisotropic counterstreaming system of forward-directed, laser-accelerated fast electrons and current-neutralizing, cold plasma electrons, that is a Weibel-like current filamentation instability. Further, while the growth of magnetic-field fluctuations by the Weibel-like filamentation current instability was reported in [3] and discussed in an ex-

perimental context in [4] in absence of collisional ionization, the generation of Weibel-like magnetic field structures is universal and consistently seen in all our CALDER Particle-In-Cell simulations over a broad range of numerical and physical parameters, both with and without collisional ionization. However, the quantitative integrated $B$-field and the timescale of its evolution might have dependence with these physical effects, in particular collisional ionization, and the systematic study of the quantitative effect is beyond the scope of this paper and will be the object of a future article.

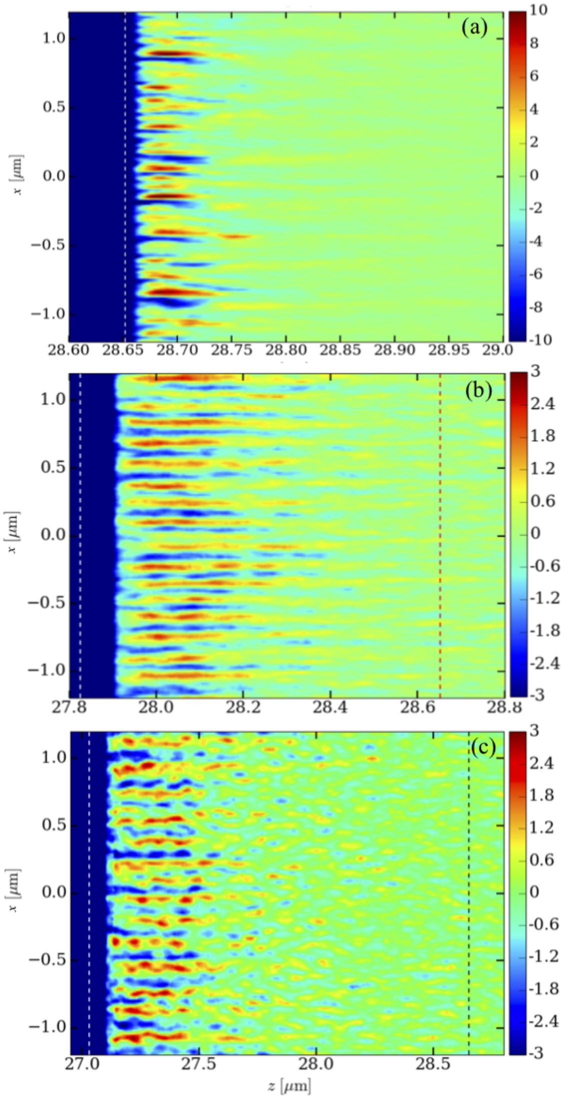


Figure 1: 2D high resolution (now with longitudinal cell size of $\lambda_0/400$) simulations showing Weibel-like magnetic field filament generation for different preplasma lengths of (a) 0 $\mu$m or flat surface/sharp density gradient (b) a linear ramp of $\lambda_0$ and (c) a linear ramp of $2\lambda_0$ for $a_0 = 2.3$ case after 20 fs of laser peak arrival at the surface of the foil. The colorbar depicts the $B$-field in units of kT. The two vertical lines show the start and end of the initial unperturbed preplasma.

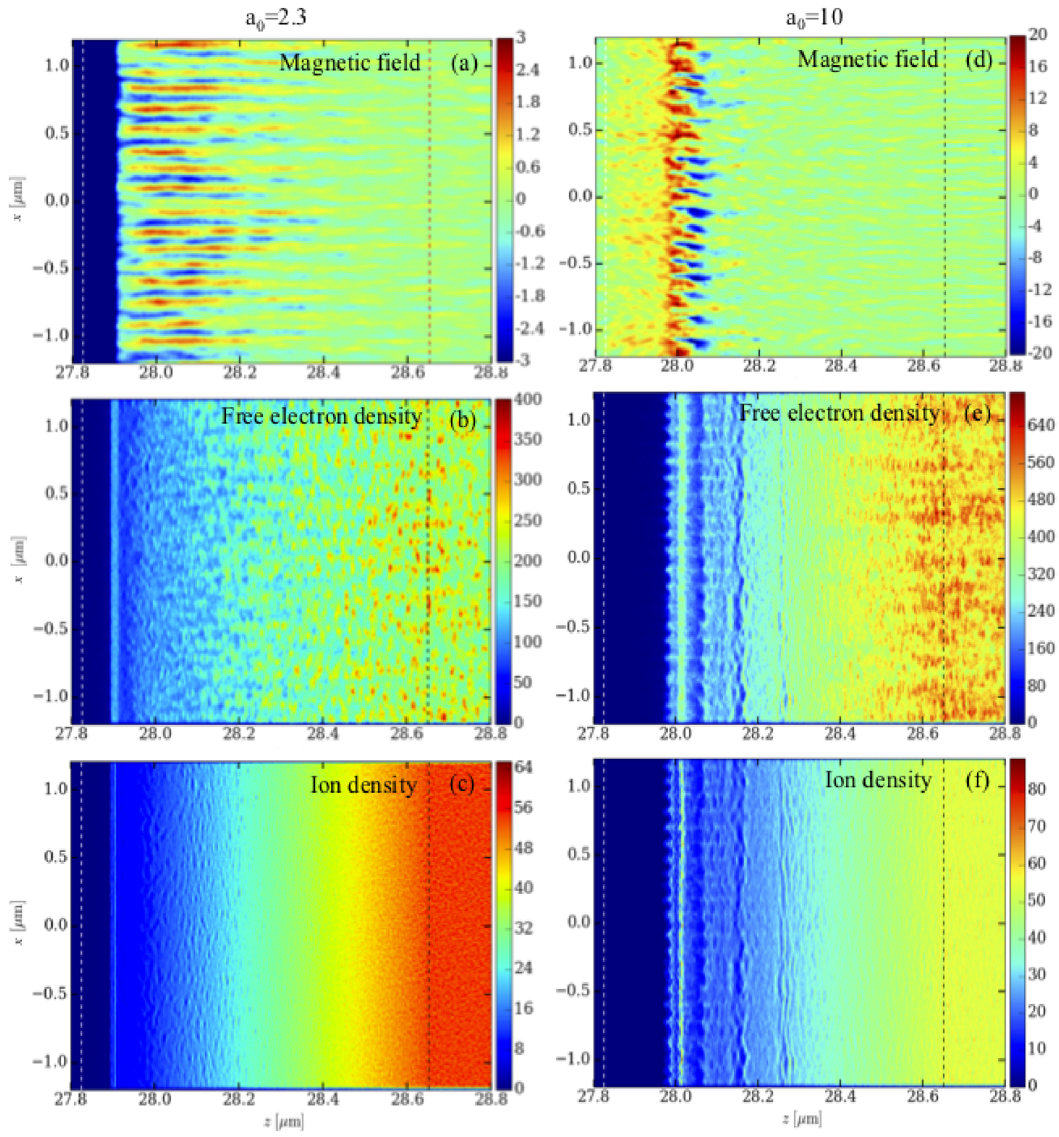


Figure 2: 2D high resolution (now with longitudinal cell size of $\lambda_0/400$) simulations, comparing low ($a_0 = 2.3$) & high ($a_0 = 10$) intensity laser interaction with the aluminium foil after 20 fs of laser peak arrival at the surface of the foil; where (a) and (d) show the generated magnetic fields (in units of kT); (b) and (e) show the total free electron densities ($n_e/n_c$) while (c) and (f) show the ion densities ($n_i/n_c$) for the 2 cases. The two vertical lines show the start and end of the initial unperturbed preplasma.

## References

[1] J. Metzkes, T. Kluge, K. Zeil, M. Bussmann, S. D. Kraft,T. E. Cowan, and U. Schramm, New J. Physics **16**, 023008 (2014).

[2] T. Kluge, J. Metzkes, K. Zeil, M. Bussmann, U. Schramm, and T. E. Cowan, Phys. Plasmas **22**, 064502 (2015).

[3] Y. Sentoku, K. Mima, S. Kojima, and H. Ruhl, Phys. Plasmas **7**, 689 (2000).

[4] S. Mondal *et al.*, Proc. Natl. Acad. Sci. **109**, 8011 (2012).
